# Supplementary material for: sEEG-based Encoding for Sentence Retrieval: A Contrastive Learning Approach to Brain-Language Alignment
Source: arXiv:2504.14468 source file (2025-04-20)
Supplement: Supplementary file 1 [file X_suppl.tex]

\clearpage
\setcounter{page}{1}
\maketitlesupplementary

% \section{Data Augmentation Strategies}
% \label{sec:data_augmentation}

% \subsection{Electrode Masking}
% \begin{algorithm}[H]
% \caption{Electrode Masking}
% \begin{algorithmic}[1]
% \Require Input tensor $x \in \mathbb{R}^{B \times E \times C \times F \times T}$, mask ratio $r$
% \For{$b = 1$ to $B$}
%     \State Sample $M = \lfloor r \cdot E \rfloor$ random electrode indices
%     \State Set $x[b, \text{masked electrodes}, :, :, :] = 0$
% \EndFor
% \Ensure Masked tensor $x$
% \end{algorithmic}
% \end{algorithm}

% \subsection{Time-Frequency Masking}
% \begin{algorithm}[H]
% \caption{Time-Frequency Masking}
% \begin{algorithmic}[1]
% \Require Input tensor $x \in \mathbb{R}^{B \times E \times C \times F \times T}$, frequency mask ratio $r_f$, time mask ratio $r_t$
% \For{$b = 1$ to $B$}
%     \If{$r_f > 0$}
%         \State Sample $M_f = \lfloor r_f \cdot F \rfloor$ random frequency indices
%         \State Set $x[b, :, :, M_f, :] = 0$
%     \EndIf
%     \If{$r_t > 0$}
%         \State Sample $M_t = \lfloor r_t \cdot T \rfloor$ random time indices
%         \State Set $x[b, :, :, :, M_t] = 0$
%     \EndIf
% \EndFor
% \Ensure Masked tensor $x$
% \end{algorithmic}
% \end{algorithm}
